# Supplementary material for: Interactive Character Control with Auto-Regressive Motion Diffusion Models
Source: arXiv:2306.00416 source file (2024-08-16)
Supplement: Supplementary file 1 [file appendix.tex]

\appendix
\section{Hierarchical Control}
\section{Motion Modeling}
